# Supplementary material for: VDPP: Video Depth Post-Processing for Speed and Scalability
Source: arXiv:2604.06665 source file (2026-04-21)
Supplement: Supplementary file 1 [file supple.tex]

% supp.tex

\documentclass[10pt,twocolumn,letterpaper]{article}

\usepackage[review]{cvpr} % 제출용 (Paper ID 표시됨)

 % *** Enter the Paper ID here

% 메인 논문과 동일한 설정을 위해 preamble을 불러옵니다.
\input{preamble}

\definecolor{cvprblue}{rgb}{0.21,0.49,0.74}
\usepackage[pagebackref,breaklinks,colorlinks,allcolors=cvprblue]{hyperref}

%%%%%%%%% PAPER ID - 메인 논문과 동일하게 설정
% \def\paperID{10811} 
% \def\confName{CVPR}
% \def\confYear{2026}

%%%%%%%%% TITLE - 보충 자료용 제목
% \title{Supplementary Material for VDPP: Video Depth Post-Processing \\for Speed, Coherence, and Plug-and-Play Scalability}

\begin{document}
% \maketitle

% --- 서플리멘터리 전용 설정 시작 ---
% 페이지 번호, 그림 번호 등을 초기화하고 'S'를 붙여 구분합니다.
\setcounter{section}{0}
\setcounter{figure}{0}
\setcounter{table}{0}
\setcounter{equation}{0}
\setcounter{page}{1}

% 섹션 번호를 알파벳(A, B...)으로 변경
\appendix

% 그림/표 번호 앞에 'S' 붙이기 (예: Figure S1)
% \renewcommand{\thefigure}{S\arabic{figure}}
% \renewcommand{\thetable}{S\arabic{table}}
% \renewcommand{\theequation}{S\arabic{equation}}
% --- 서플리멘터리 전용 설정 끝 ---

% 실제 Appendix 내용 불러오기
\input{sec/x_appendix}

% 만약 Appendix 내에도 인용(Citation)이 있다면 아래 줄 필요
{
    \small
    \bibliographystyle{ieeenat_fullname}
    \bibliography{main}
    \clearpage
}

\end{document}
